# Supplementary material for: Optimization of Forcemyography Sensor Placement for Arm Movement Recognition
Source: arXiv:2207.10915 source file (2022-07-22)
Supplement: Supplementary file 1 [file 6-appendix.tex]

\section*{APPENDIX}
